# Supplementary material for: Fast Similarity Sketching
Source: arXiv:1704.04370 source file (2024-05-05)
Supplement: Supplementary file 1 [file appendix.tex]

\section{Proof of \texorpdfstring{\Cref{lem:separate}}{the separation lemma}}
\label{sec:separateproof}

\begin{proof}
For $i = 0,1,2,\ldots,n$ we let $X_{<i} = \sum_{j < i} X_j$.

First we prove the bound on the expected value of $\tau_F$. For $j = r,r+1,\ldots,t$
let $T_j = j$ if the algorithm returns \false{} when $i=j$ in the loop and let
$T_j = 0$ otherwise. We clearly have that $\tau_F = r + \sum_{i=r}^t T_i$.
Clearly $\sum_{i=r}^{2r} T_i \le 2r$ by definition, and therefore
\begin{align*}
	\tau_F \le 3r + \sum_{i = 2r+1}^t T_i
	\, .
\end{align*}
Now fix $i > 2r$. If $T_i = i$ then we must have that $X_{<i} \ge i \cdot
    \gamma + \sqrt[3]{i^2}$.
Let $j = \floor{i/2}$. Since the algorithm did not stop earlier we must also have
    $X_{<j} < j \cdot \gamma + \sqrt[3]{j^2}$. Hence we have that:
\begin{align*}
	\Ep{T_i} \le 
	i \cdot \min \set{
		\Prp{X_{<i} \ge i \cdot \gamma + \sqrt[3]{i^2}},
		\Prp{X_{<j} < j \cdot \gamma + \sqrt[3]{j^2}}
	}
	\, .
\end{align*}
Let $\gamma' = \gamma + \frac{1}{2} \cdot \left ( \frac{1}{\sqrt[3]{i}} + \frac{1}{\sqrt[3]{j}} \right )$.
If $p \le \gamma'$ then we see that if $X_{<i} \ge i \cdot \gamma +\sqrt[3]{i^2}$ then:
\begin{align*}
    X_{<i} - \Ep{X_{<i}} \ge 
	i \cdot \gamma + \sqrt[3]{i^2} - i \gamma'
	= \Omega \left ( \sqrt[3]{i^2} \right )
	\, .
\end{align*}
And by Hoeffding's inequality we conclude that:
\begin{align*}
    \Prp{X_{<i} - \Ep{X_{<i}} \ge i \cdot \gamma + \sqrt[3]{i^2} - i \gamma'}
	\le 
	e^{-\Omega(\sqrt[3]{i})}
	\, .
\end{align*}
%We note that Hoeffding's inequality holds by the same reasoning as
%in \Cref{lem:chernoffLemma}.
If $p > \gamma'$ we conclude in the same manner that
$\Prp{X_{<j} < j \cdot \gamma + \sqrt[3]{j^2}} \le e^{-\Omega(\sqrt[3]{i})}$.
Hence we get that:
\begin{align*}
	\Ep{\sum_{i = 2r}^t T_i}
	\le 
	\sum_{i=2r}^t i \cdot e^{-\Omega(\sqrt[3]{i})}
	\le 
	\sum_{i \ge 1} i \cdot e^{-\Omega(\sqrt[3]{i})}
	= O(1)
	\, .
\end{align*}
We conclude that $\Ep{\tau_F} = O(r)$ as desired.

We now assume that $p \ge \gamma + \delta$ and prove that \eqref{eq:probLargeJ} is
a lower bound on the probability that \true{} is returned.
By a union bound and Hoeffding's inequality we get that the probability that
\false{} is returned is at most
\begin{align*}
	\sum_{i = r}^t
		\Prp{X_{< i} \le i \cdot \gamma + \sqrt[3]{i^2}}
	& \le
	\sum_{i = r}^t
		\Prp{X_{< i} \le i \cdot (\gamma + \delta/2)}
	\\
	& \le
	\sum_{i = r}^t
		\Prp{X_{< i} - \Ep{X_{<i}} \le -i \cdot \delta/2}
	\\
	& \le 
	\sum_{i = r}^t
		e^{-\delta^2 i/2}
	\\
	& \le 
	\sum_{i \ge r}
		e^{-\delta^2 i}
	=
	\frac{e^{-\delta^2 r/2}}{1-e^{-\delta^2/2}}
	\, ,
\end{align*}
as desired.

Now assume that $p \ge \gamma - \delta$. We note that \true{} is only returned
if $X_{<t} > t \cdot \gamma$. By Hoeffding's inequality this happens with
probability at most
\begin{align*}
	\Prp{X_{<t} > t \cdot \gamma + \sqrt[3]{t^2}}
	\le 
	\Prp{X_{<t} > t \cdot \gamma}
	\le 
	\Prp{X_{<t} - \Ep{X_{<t}} > t \cdot \delta}
	\le
	e^{-2\delta^2 t}
	\, ,
\end{align*}
showing that \eqref{eq:probSmallJ} holds.
\end{proof}
